# Supplementary material for: Detectability of core level crossing and electronic topological transformations: the case of Osmium
Source: arXiv:2204.10057 source file (2022-08-08)
Supplement: Supplementary file 1 [file Supplementary.pdf]

# Detectability of core level crossing and electronic topological transformations: the case of Osmium

Gavin A. Woolman and Graeme J. Ackland<sup>1\*</sup>

<sup>1</sup>Centre for Science at Extreme Conditions and School of Physics and Astronomy, University of Edinburgh, Edinburgh, U.K.

## WIEN2K CALCULATION DETAILS

A large series of calculations were done with several different functions using two different *ab initio* codes. Calculations were conducted for unit-cells with a dense array of volumes ranging between 17 and 29.4 Å<sup>3</sup>, and with a series of different  $c/a$  ratios ranging from 1.565 to 1.615 at 0.025 steps for the PBE calculations, and between 1.56 and 1.615 for the calculations using SCAN and LDA. We note that SCAN is implemented non-selfconsistently in Wien2k. Figure 1 illustrates the density of points calculated. *Ab initio* calculations of the total energy were conducted on this dense grid of  $c/a$  and volumes. The  $c/a$  ratio minimizing energy at constant volume was then found for each individual volume.

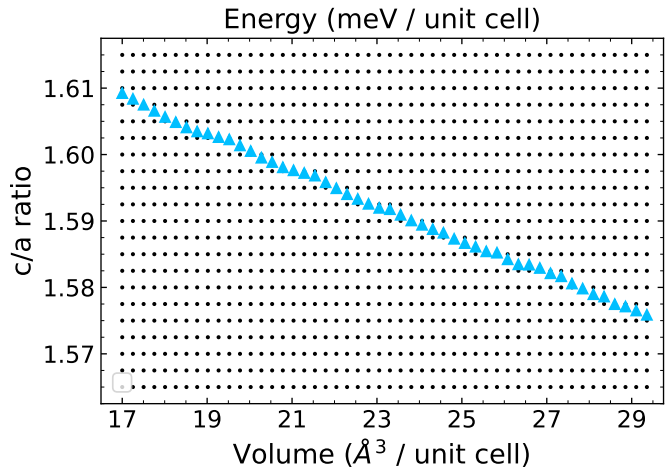

FIG. 1: Solid dots show the combinations of  $c/a$  ratio and volume used in the energy calculations for the calculations using the PBE exchange-correlation potential. The  $c/a$  ratio which minimizes energy at constant volume is also shown as blue triangles.

Three approximations for the exchange and correlation effects were considered: the local-density approximation (LDA)[1], the generalized gradient approximation as implemented by Perdew, Burke, and Ernzerhof (PBE)[2], and the meta-generalized gradient approximation by Sun *et al.* (SCAN)[3].

Calculations were conducted using the all-electron augmented-plane-wave with local-orbitals, (L)APW+lo, method as implemented by the Wien2k code (Wien2k 21.1)[4]. The radius of the atomic-sphere muffin-tins  $R_{\text{MT}}$  was set to  $2.13 a_0$ . This value is smaller than the default in order to prevent the muffin-tins overlapping at the small volumes we needed to compute. The  $5s$ ,  $5p$ ,  $4f$ ,  $5d$ , and  $6s$  orbitals were treated as valence states, and allowed to extend outside the muffin tins. Regular Monkhorst-Pack  $50 \times 50 \times 30$  grids of  $k$ -points were used for Brillouin-zone sampling for the PBE and SCAN, and for the LDA potential a  $40 \times 40 \times 22$  grid was used. These grids were denser than convergence tests suggested were necessary, in order to ensure any electronic topological transitions were accurately sampled.

The largest Kohn-Sham plane-wave vector,  $K_{\text{max}}$ , was given by  $R_{\text{MT}} \times K_{\text{max}} = 10.0$  for PBE and SCAN functionals, and 9.0 for the LDA functional, and tested for convergence. The magnitude of the largest vector used in the charge-density Fourier expansion was set to  $G_{\text{max}} = 20 a_0^{-1}$ . These parameters were greater than convergence tests indicated necessary, in order to ensure small perturbations could be accurately calculated and numerical noise due to finite basis size was minimized.

Spin-orbit coupling was included. Including this required additional high-energy states to be computed. The highest energy above the Fermi-energy involved in the computation,  $E_{\text{max}}$ , was increased to 13 Ry. The exact energies of the local orbitals also had to be adjusted from the defaults in order to prevent ghost bands. Failure to make these changes

caused errors in the low volume region (below  $\sim 19 \text{ \AA}^3/\text{uc}$ ). The parameters for the local orbitals can be most easily expressed by showing an example `case.in1` input file, shown below:

```
WFFIL EF=1.24464979901203433540 (WFFIL, WFPRI, ENFIL, SUPWF)
 10.00 10 4 ELPA pxq BL 64 (R-MT*K-MAX,MAX L IN WF,V-NMT,LIB)
 0.30 7 0 (GLOBAL E-PARAMETER WITH n OTHER CHOICES, global APW/LAPW)
0 1.46 0.0000 CONT 1
0 -6.41 0.0001 STOP 1
1 1.75 0.0000 CONT 1
1 -3.20 0.0001 STOP 1
3 1.76 0.0000 CONT 1
3 -3.39 0.0001 STOP 1
2 1.68 0.0010 CONT 1
K-VECTORS FROM UNIT:4 -10.0 13.0 62 emin / de (emax=Ef+de) / nband
```

# TOPOLOGICAL TRANSITIONS

The calculated bandstructure of osmium is very similar for all three exchange-and-correlation potentials (Fig. 2). Figure 3 shows a comparison between our calculated Fermi surface and the Fermi surface measured by Kamm & Anderson using the de Haas–van Alphen method. Figure 4 shows how the energy of special points in the bandstructure, relative to the Fermi energy at  $\Gamma$  and  $L$  change under pressure.

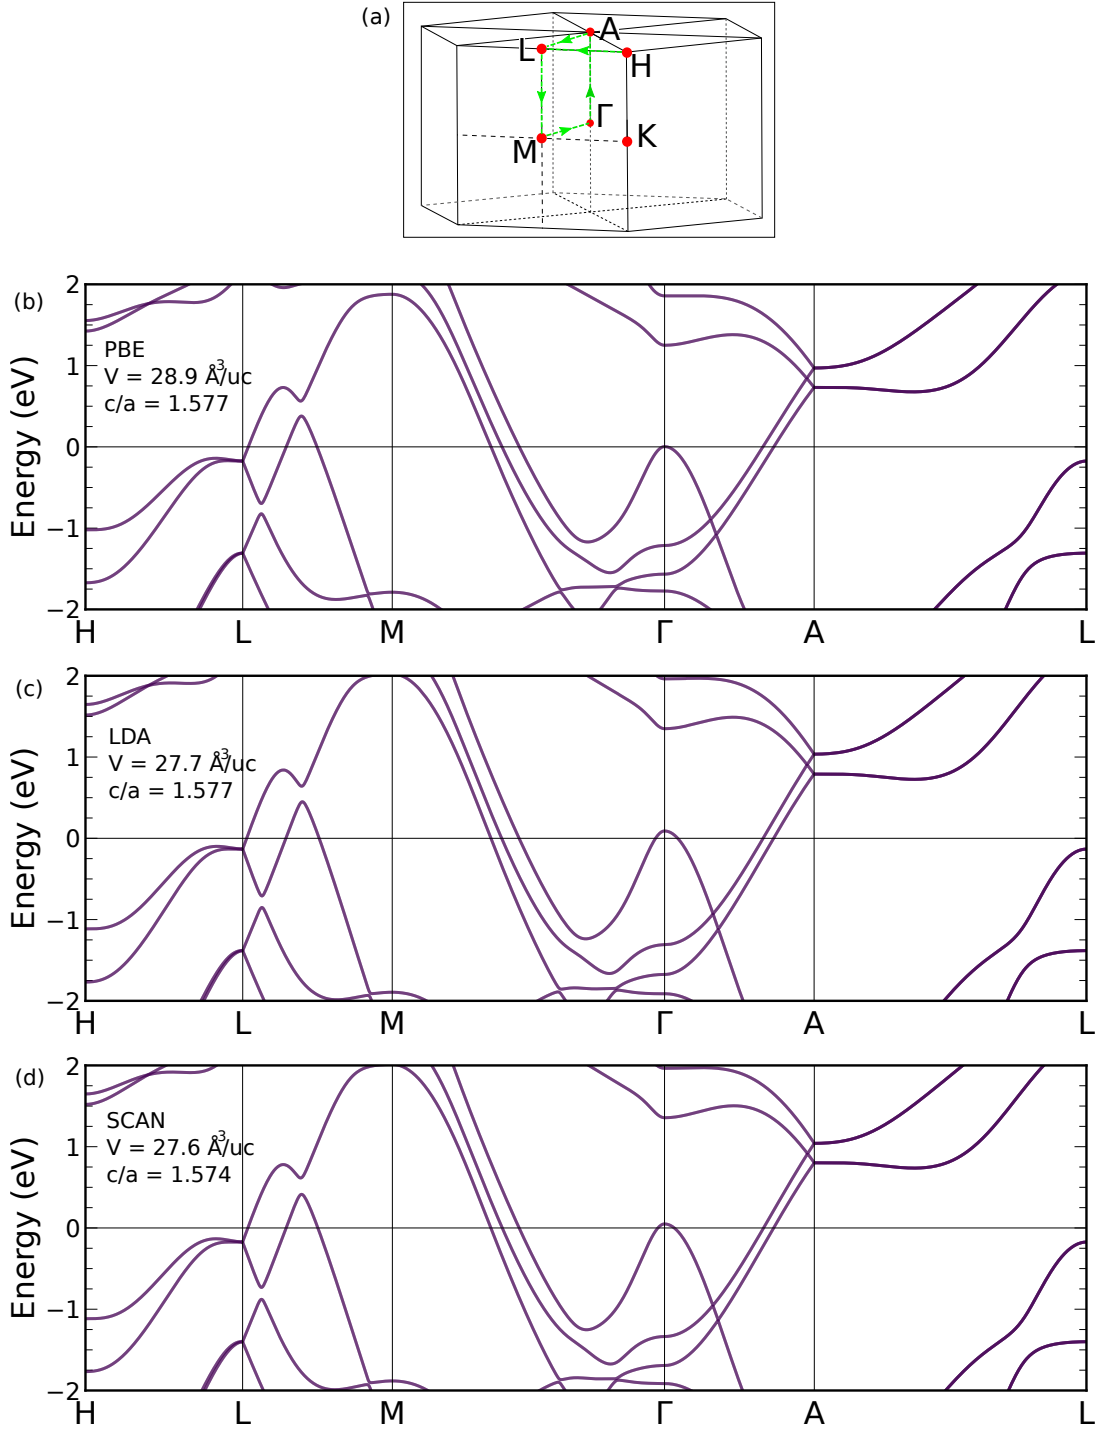

FIG. 2: Bandstructure of osmium calculated using the (b) PBE, (c) LDA, (d) SCAN exchange-and-correlation energy, at volumes and  $c/a$  ratios close to the fitted zero-pressure values. (a) A diagram of the Brillouin-zone path examined.

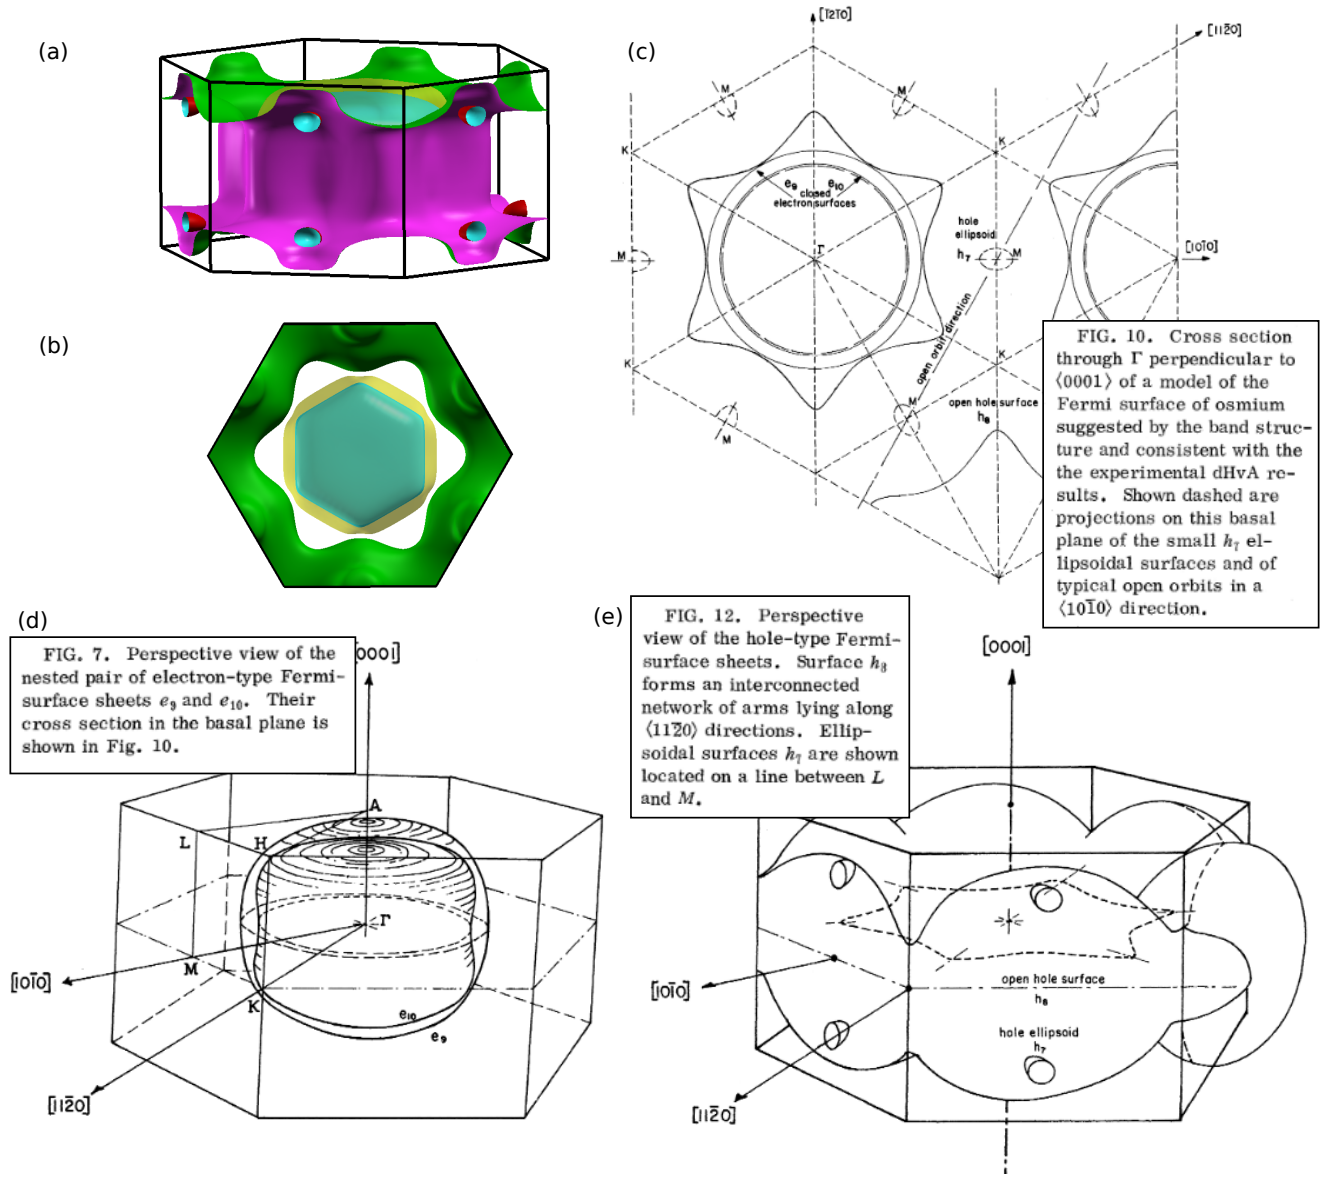

FIG. 3: Comparison between calculated Fermi surface and de Haas–van Alphen measurements taken from Kamm & Anderson (1970)[5]. (a) & (b) views of the calculated Fermi surface, calculated using the PBE exchange-correlation potential. (c)–(e): figures taken from Kamm & Anderson of the experimentally measured Fermi surface from different perspectives.

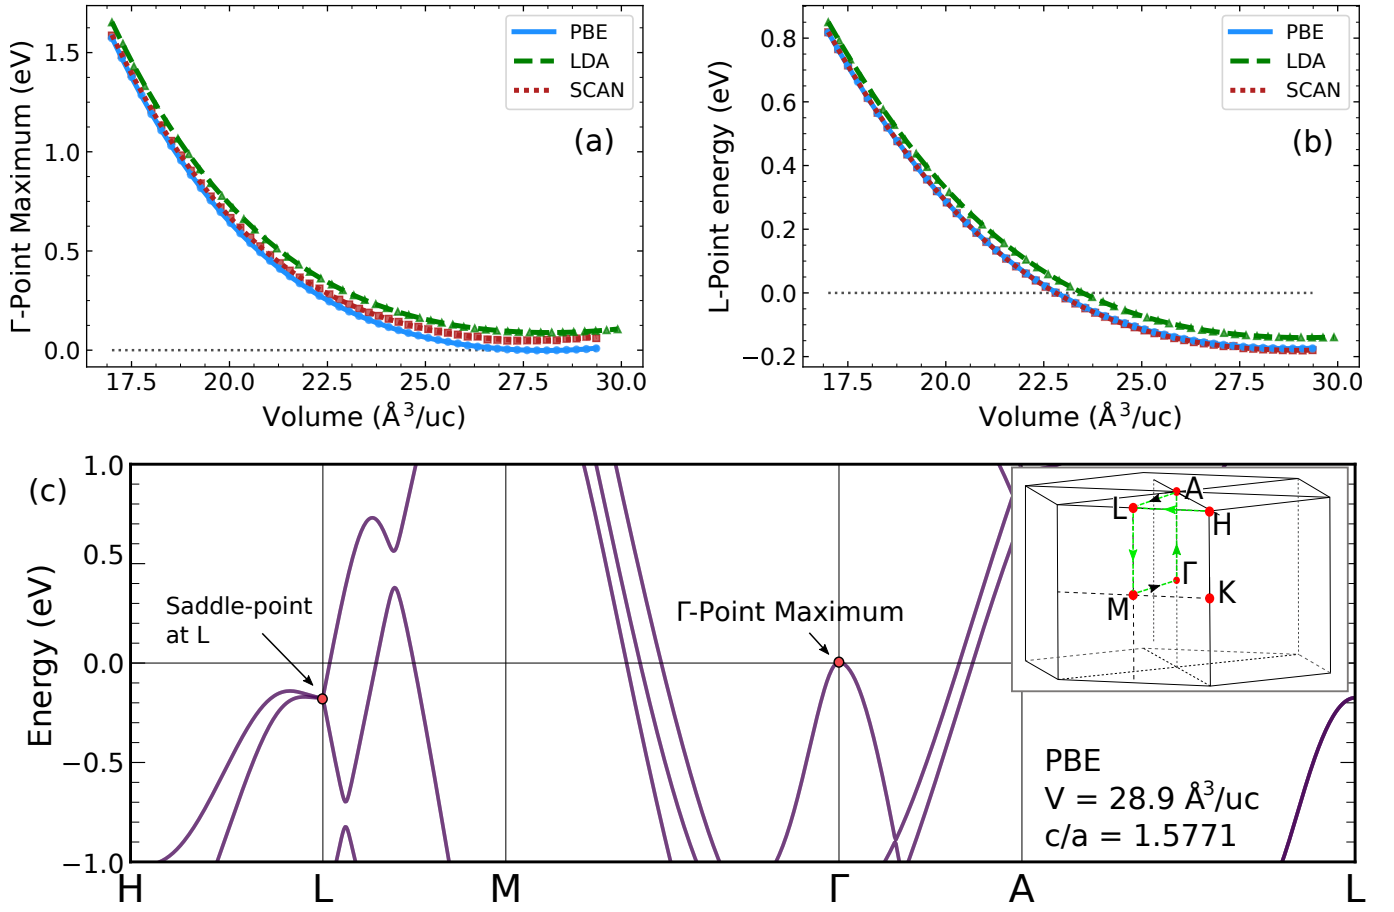

FIG. 4: Energy of the (a) valence-band maximum at  $\Gamma$ , (b) saddle-point at  $L$ , against volume for the three different exchange-correlation potentials used. Symbols are data-points, lines are guides to the eye. The  $c/a$  ratio at each volume is always the ratio which minimizes energy for that volume and exchange-correlation potential. (c) Bandstructure of osmium, calculated using the PBE exchange-correlation potential, with special points labelled.

# EQUATION OF STATE OF OSMIUM FITS

The Birch-Murnaghan equation gives an excellent fit to the calculated data for all exchange-correlation potentials, as shown by the small residuals [Fig. 5]. The underlying calculation is deterministic and the equation is analytic, so there are no stochastic errors. No discontinuity in the equation of state can be detected: the cusp in the residuals can be traced to the change in size of a discrete grid in Wien2k. There is not a consistent kink in the residuals which could be associated with the L-point transition.

The equation of state fits do not include the final few points, which are ignored due to a discontinuous jump in the energy caused by a change in the finite basis set. This discontinuous jump can be seen in the residuals. A reduction in the radius of the muffin tins, which in turn changes the augmented-plane-wave basis set, removes this discontinuity but does not change the volume at which core-hybridisation sets in. Having confirmed that the discontinuity is a computational anomaly, and not due to core-hybridisation, and because the full span of  $c/a$  and volume calculations was very time intensive, we chose not to repeat the entire set of calculations with a smaller muffin-tin radius.

The equations of state for all three functionals are broadly similar, with the primary difference being the zero pressure volume  $V_0$  (Fig. 6).

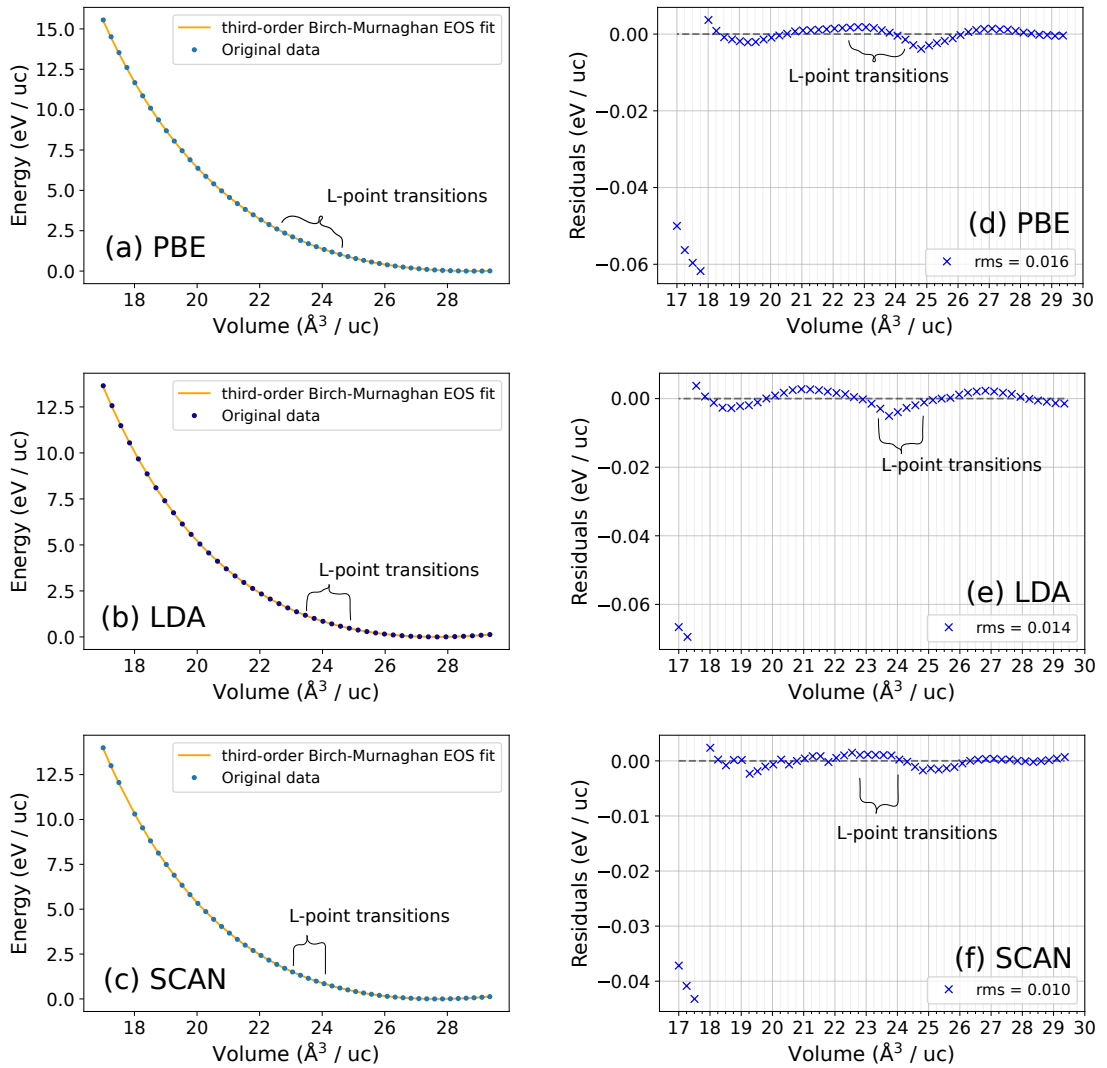

FIG. 5: Third-order Birch-Murnaghan equation of state fits for all three functionals. (a)–(c) Fit of the calculated total energy as a function of volume, (d)–(f) residuals of the fits. Windows over which the electronic topological transitions in the vicinity of the L-point take place are shown. The discontinuities in the residuals are associated with a discontinuous change in the finite basis set. These jumps disappear if a smaller muffin-tin radii is used.

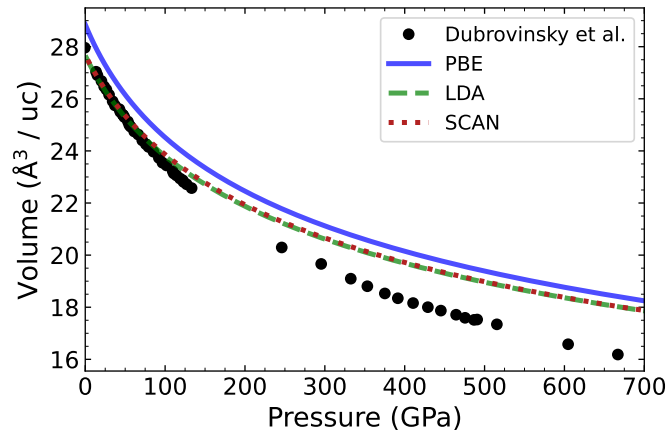

FIG. 6: Calculated equations of state for the LDA, PBE, and SCAN exchange-correlation energy, fitted to a third-order Birch–Murnaghan equation, alongside the XRD datapoints of Dubrovinsky *et al.*[6]

ENERGY,  $c/a$ , AND VOLUME.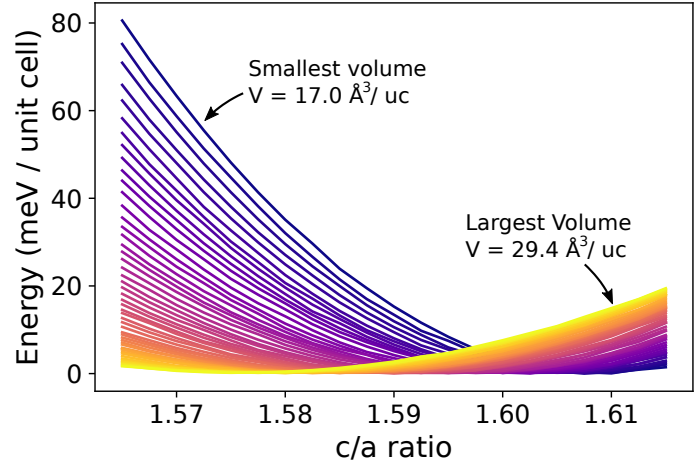

FIG. 7: Energy as a function of  $c/a$  ratio at constant volume for all volumes considered. This is for the PBE exchange–correlation potential. The energies of each curve have been shifted such that the minimum energy at each volume is zero.

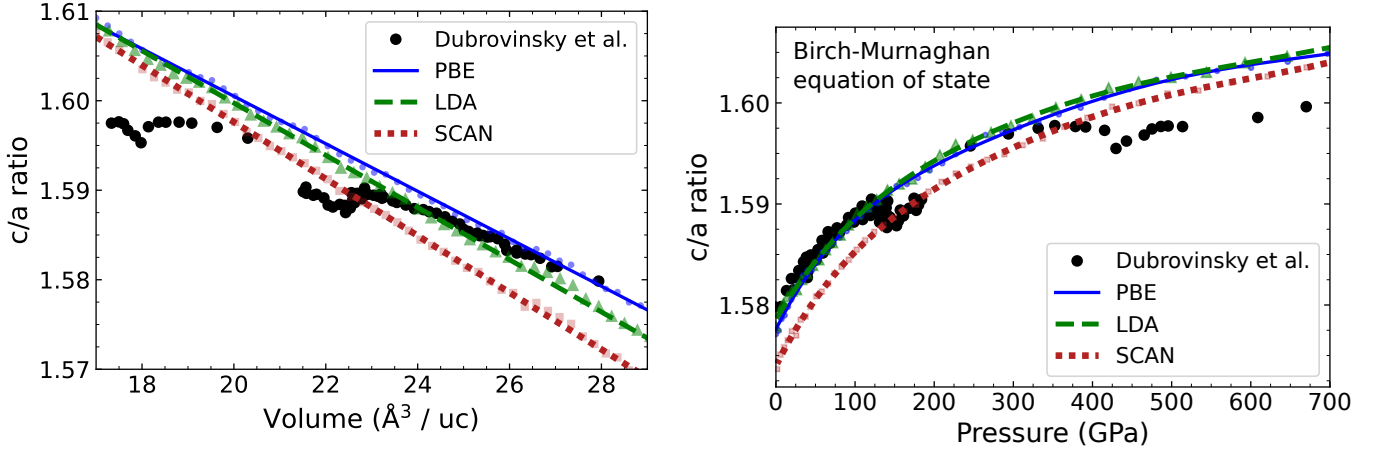

FIG. 8: Left: Optimal  $c/a$  ratio against volume for all three exchange–correlation potentials used in this work. Calculations used the Wien2k code. Symbols are datapoints, lines are linear fits used as guides for the eye. Experimental results from Dubrovinsky *et al.*[6] are also shown. Right:  $c/a$  ratio which minimizes the energy at constant volume, against pressure. Symbols are datapoints, lines are guides to the eye. Third-order Birch–Murnaghan equation of states, fitted to energy as a function of volume, were used to calculate the pressure of each calculated data-point.

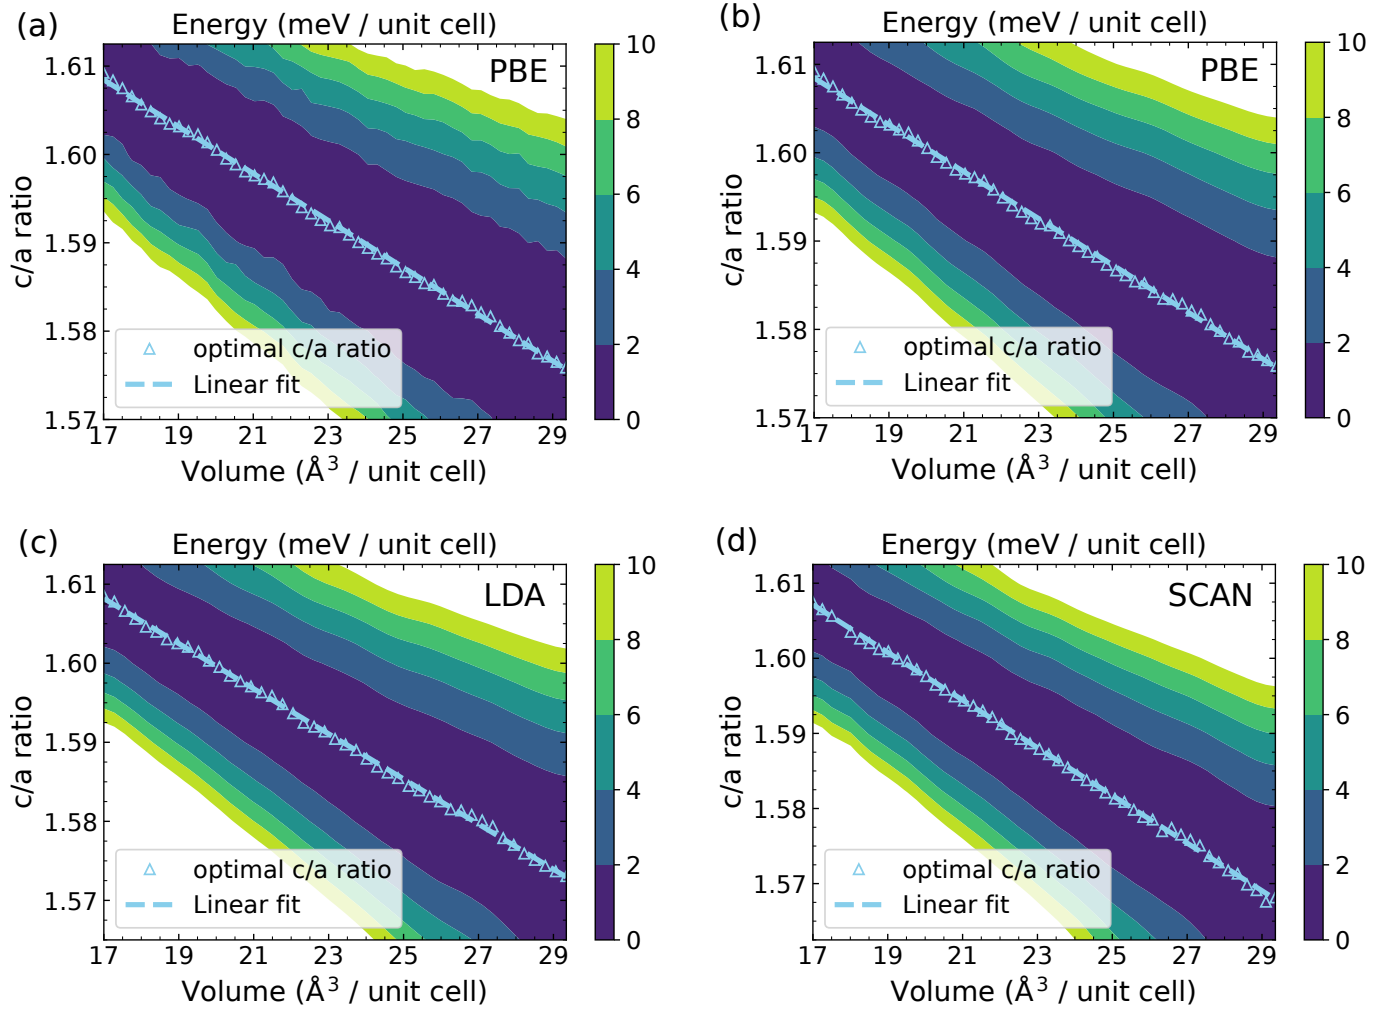

FIG. 9: Contour plots of energy against  $c/a$  ratio and volume, calculated using (a) & (b) the PBE exchange-correlation potential, (c) LDA, (d) PBE with SCAN geometry. At each volume, energy as a function of  $c/a$  was shifted so that the minimum energy was at zero: this was done purely to ease contour plotting. To find the optimal  $c/a$  ratio at each volume which minimizes the energy (blue triangles), a parabola was fitted to the eight lowest energy points at that volume. (a) No smoothing has been applied; (b), (c), (d) gaussian smoothing has been applied.

# COUPLING OF L-POINT CROSSOVER TO $c/a$ AND THE TOTAL ENERGY

If an ETT causes an anomaly in the hydrostatic  $c/a$  ratio of osmium, one would expect that energy of points in the bandstructure associated with this ETT would incur discontinuous or anomalous perturbations when  $c/a$  is varied. Figure 10(a) shows the energy of the L-point crossing as a function of  $c/a$  at a constant volume. As  $c/a$  is increased, the energy of the band-crossing at L smoothly increases, with no anomalies or discontinuities as it passes through the Fermi energy. This shows that the ETT has no anomalous effect on the bandstructure — suggesting it is unlikely there is any change to the bonding or crystal structure.

Furthermore, Fig. 10(b) shows the total energy as a function of  $c/a$ . There is no significant deviations that can be associated with the L-point ETT: indeed, the total energy vs  $c/a$  curve is remarkably well described by a simple parabola. This shows that the ETT does not cause any perturbations in the zero-temperature bandstructure. In addition, the smoothness of the curve in Fig. ??(b) suggests the ETT holds no significance on the elastic constants and other properties which derive from the elastic constants, such as phonon-spectra and thermal expansion coefficients.

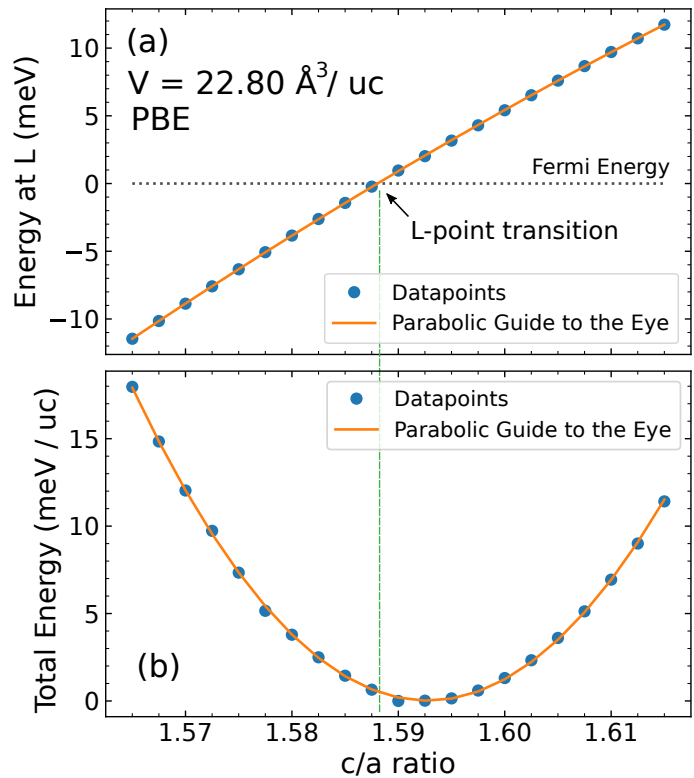

FIG. 10: (a) Energy at the L-point against  $c/a$  at constant volume. Calculations used the Wien2k code with the PBE exchange-correlation potential. (b) Total energy vs  $c/a$  at constant volume. As shown, there is no discontinuities or perturbations in the neighbourhood of the L-point ETT. Indeed, the total energy vs  $c/a$  is remarkably well described by a parabolic fit, as is the energy at L vs  $c/a$ .

### COUPLING OF THE DOS TO $c/a$ RATIO

If one expects the hybridisation of core-level orbitals to cause anomalies in the  $c/a$  ratio under pressure, one should also expect that artificially straining the  $c/a$  ratio at constant volume should have visible effects on the density of states at these core levels. At a volume of  $17.0 \text{ \AA}^3/\text{uc}$ , using the PBE exchange-correlation potential, the lowest energy  $c/a$  ratio is 1.609. Figure 11 shows that changing the  $c/a$  ratio between 1.600 and 1.615, while holding the volume constant, causes negligible changes to the density of states. This change in  $c/a$  is roughly three times greater than the perturbations seen by Dubrovinsky *et al.*[6]. Given there appears to be negligible coupling between  $c/a$  and the  $4f_{7/2}$  and  $5p_{3/2}$  orbitals, it is unlikely core-level hybridisation could have caused the anomalies seen by Dubrovinsky *et al.*.

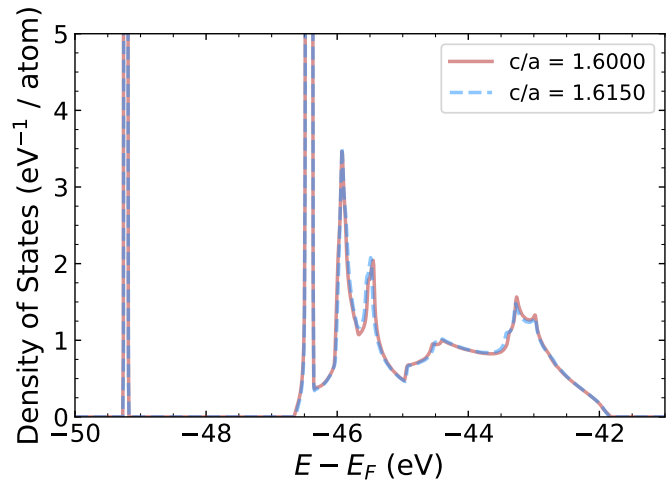

FIG. 11: Density of states for  $5p_{3/2}$  core electrons with  $V = 17.0 \text{ \AA}^3/\text{uc}$  with two different  $c/a$  ratios.

## VASP CALCULATIONS

### VASP calculation methodology

One set of calculations were conducted using the Vienna *ab-initio* simulation package (VASP version 5.4.4[7][8]). Exchange and correlation effects were computed using the generalized gradient approximation as implemented by Perdew, Burke, and Ernzerhof[2], and the local density approximation [1]. Eight valence electrons per atom were calculated, with the core electrons accounted for using the projected-augmented wave method to describe the electron-core interaction. These eight electrons should account for the  $6s^2$  and  $5d^6$  valence orbitals. The  $4f$  and  $5p$  core electrons are included in the plane-augmented-wave potential, which does not change with pressure. As a result, any changes in the crystal structure due to changing core-electron state hybridising will not be included. However, any perturbations in  $c/a$  due to electronic topological transitions should still be present.

The largest plane-wave vector used in the expansion of the Kohn-Sham orbitals was parameterized by a cut-off energy (ENCUT) of 400 eV. The full grid was used during the fast-Fourier transform steps of the calculation. A regular Monkhorst-Pack grid of  $40 \times 40 \times 40$   $k$ -points was used for Brillouin-zone sampling. This grid was denser than convergence calculations indicated was necessary, and was chosen to ensure that any topological transitions in the Brillouin zone would be well sampled. Including spin orbit coupling does change the bandstructure, however, the ETT at L is simulated with or without spin orbit coupling [Fig. 12]. Therefore, for computational efficiency, and because the Wien2k calculations all included spin-orbit coupling, we chose not to include spin-orbit coupling for the VASP calculations.

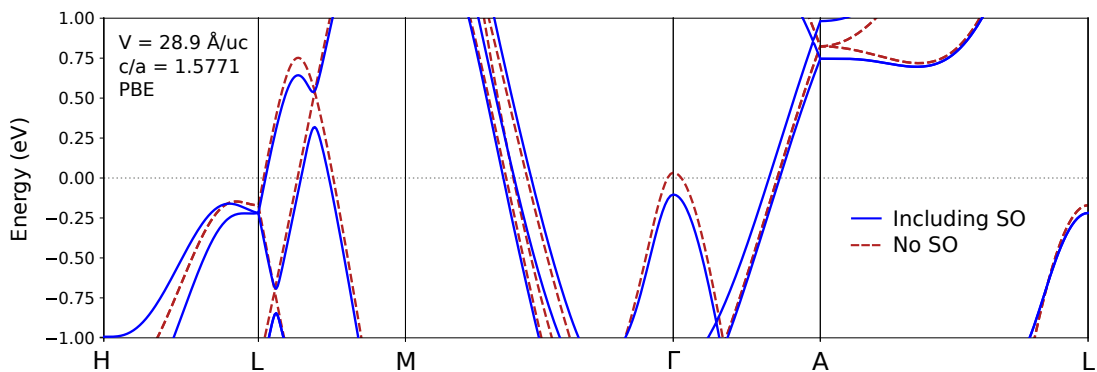

FIG. 12: Comparison of VASP bandstructures with and without spin-orbit coupling.

### Vasp Results

Figure 13 shows the total energy vs  $c/a$  ratio for several different volumes. Each curve has been shifted so that the minimum has zero energy. As shown, each volume shows a smooth curve with a unique minimum. The value of  $c/a$  which minimizes the energy increases continuously as the volume is decreased. This smooth transition is clearest in Fig. 13, which plots a curve for every volume considered.

Figure 14 shows two contour plots of energy vs  $c/a$  and volume for the set of calculations using PBE and LDA, respectively. In both cases the hydrostatic  $c/a$  increases nearly linearly with reducing volume. There are no significant perturbations or wrinkles in the energy surface which can be associated with an ETT at the L-point or at  $\Gamma$ . Indeed, residuals from a Vinet equation of state fitted to the energy vs volume data show no anomalies or discontinuities which could be associated with either ETT (Fig. 15). The root-mean-square of the residuals is less than 0.1% of the total energy difference between the lowest and highest volumes.

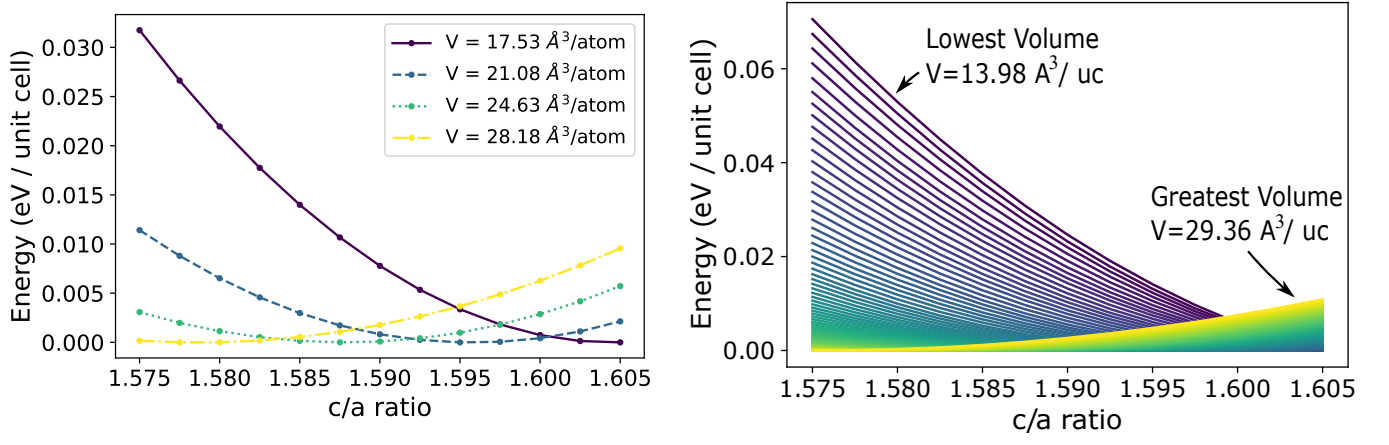

FIG. 13: Left: Total energy per unit cell vs  $c/a$  ratio at constant volume, for selected different volumes. Calculated using VASP. Right: Total energy per unit cell vs  $c/a$  ratio at constant volume, for many different volumes.

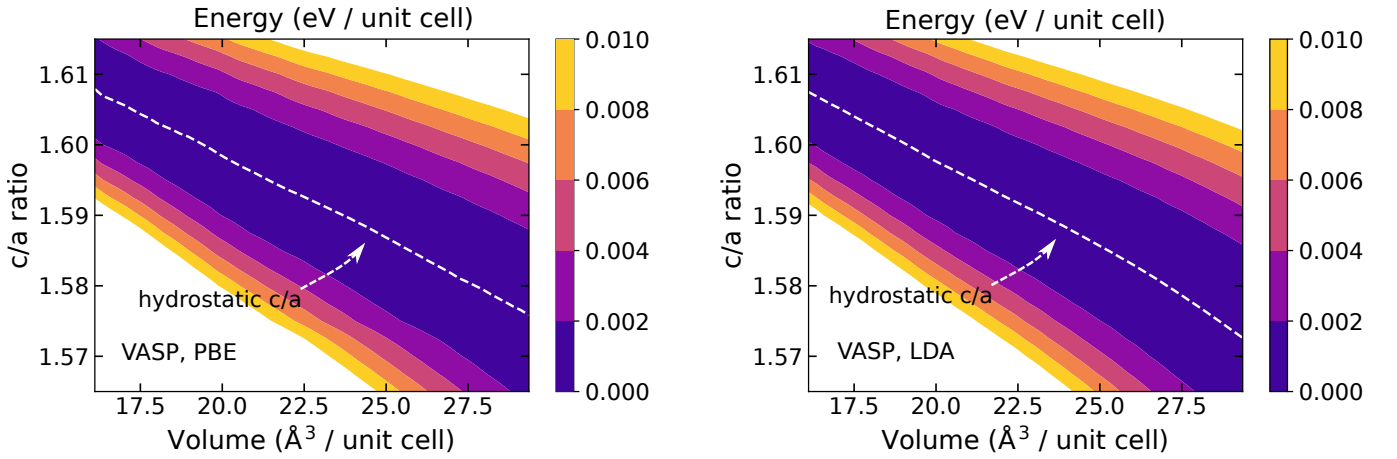

FIG. 14: Total energy per unit cell vs  $c/a$  ratio and volume. Left: PBE exchange-correlation potential, Right: LDA. For clarity, the total energy at every  $c/a$  ratio is plotted relative to the minimum energy at that volume. No smoothing was applied.

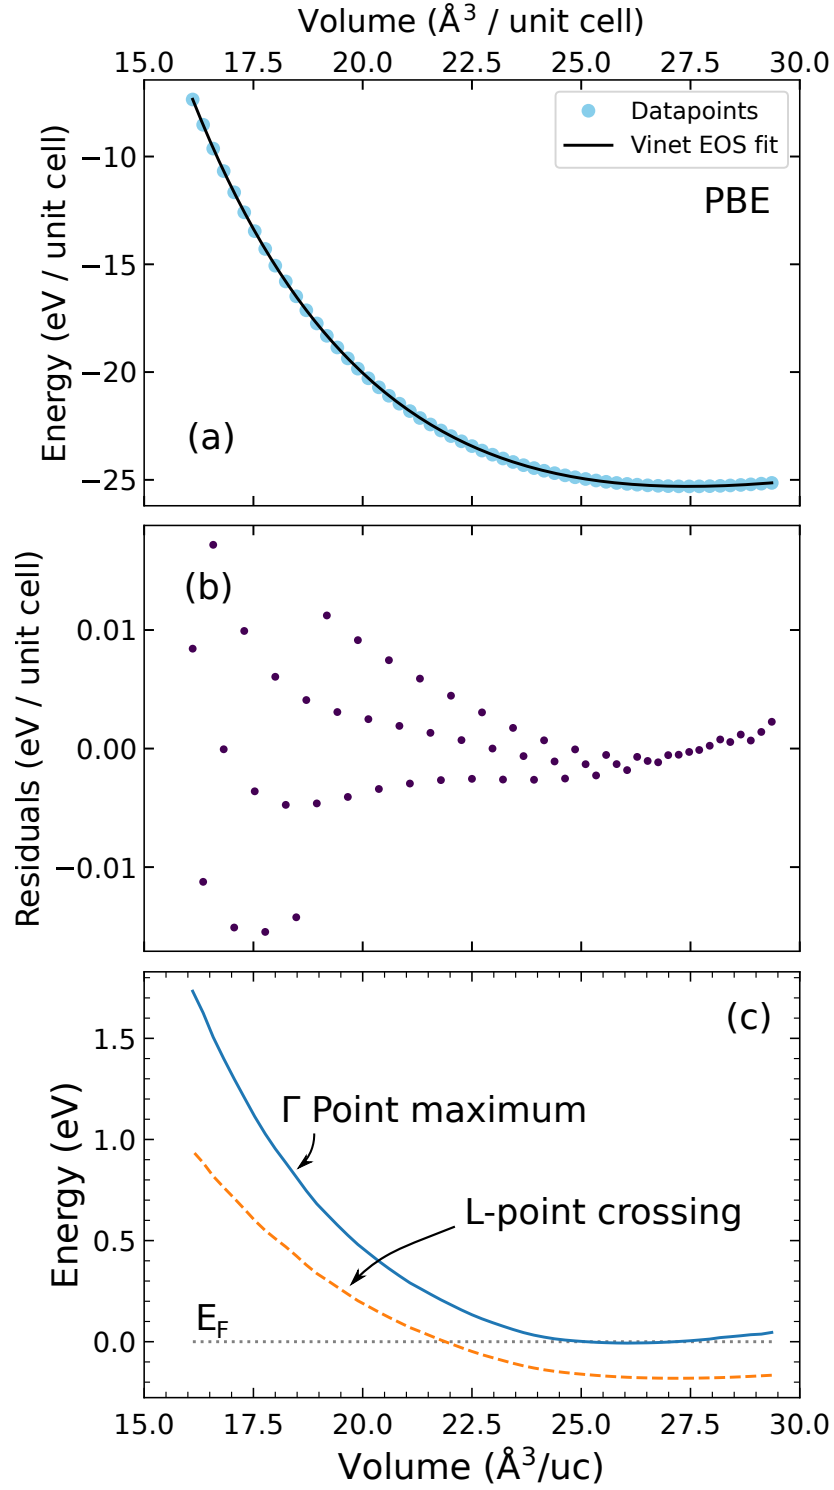

FIG. 15: (a) Total energy vs volume for the VASP calculations using PBE. The hydrostatic  $c/a$  ratio at each volume is used. A Vinet equation of state is fitted to the data. (b) Residuals of the Vinet equation-of-state fit. It is worth noting that the scale of the residuals is approximately 0.1% of the total energy scale covered. RMS = 0.006 eV. (c) Energy of the  $\Gamma$ -point maximum and  $L$ -point crossover as a function of volume.

# ANOMALIES IN THE EQUATION OF STATE

Dubrovinsky *et al.* use partial fits of the equation of state as evidence that the hybridisation of the 5p and 4f core levels having an effect on the structure of Osmium. In their words: “Fitting of the  $P$ - $V$  data by the third-order Birch–Murnaghan EOS within three pressure ranges — below 120 GPa, between 170 GPa and 400 GPa, and above 400 GPa — gives an interesting result: although fitting over the first and second pressure ranges produces similar EOS parameters ( $K_{300} = 397(3)$  GPa,  $K' = 4.07(4)$  and  $K_{300} = 416(5)$  GPa,  $K' = 3.8(1)$ , respectively...), we obtain different parameters at pressures above 400 GPa ( $K_{300} = 293(5)$  GPa,  $K' = 5.4(1)$ ). These experimentally observed peculiarities are not artefacts and require an explanation”.

The peculiarities observed may not be an artefact of the experiment. However, as we will show, it can easily be an artefact of the analysis. A simple three-parameter equation of state, such as the third-order Birch–Murnaghan, might not have the flexibility to perfectly fit data from a wide volume and pressure range. To investigate this, pressure–volume data was generated using a very simple Lennard–Jones-like equation of state:

$$E = \left( \frac{1}{V\sqrt{2}} \right)^4 - \left( \frac{1}{V\sqrt{2}} \right)^2, \quad (1)$$

$$P = 4\sqrt{2} \left( \frac{1}{V\sqrt{2}} \right)^5 - 2\sqrt{2} \left( \frac{1}{V\sqrt{2}} \right)^3, \quad (2)$$

where  $V$  is here a dimensionless quantity representing the volume. The factor of  $\sqrt{2}$  means the zero-pressure volume is  $V_{min} = 1$ . Crucially, this function is continuous and analytic for all volumes greater than zero. There are no discontinuities or anomalies in the energy function, nor the corresponding pressure function.

One hundred different volumes per atom between  $V_{min} = 1$  and 0.4 were calculated. A third-order Birch–Murnaghan equation of state was fitted to all the data, with the volume parameter  $V_0$  used as a free parameter (Fig. 16a). This gave fitting parameters  $B_0 = 0.33$ ,  $B' = 8.76$ ,  $V_0 = 1.0821$ . The fitting algorithm was very sensitive to initial parameters, and so a dense array of starting parameters was used and the best fit chosen.

The fit was then repeated on a subset of the data where the volumes were all less than 0.5 [Fig. 16(b)]. This constituted almost two thirds of the pressure range in the entire equation of state. The fitting parameters are starkly different:  $B_0 = 1.70$ ,  $B' = 5.84$ ,  $V_0 = 0.937$ . A similarly drastic change happens even if  $V_0$  is fixed [Figs. 16(c) & (d)]. Importantly, there is a drastic change in the fitting parameters  $B_0$  and  $B'$ , even though the underlying equation of state is analytic.

The issue with fitting is increased further if there is a large difference in the number of data points at low or high volumes. However, it is clear that changes in equation-of-state parameters when fitting over a subset of data, rather than the entire data-set, is completely possible without any phase transitions or discontinuities. A change in equation-of-state fitting parameters is not strong evidence of a phase transition — just that the flexibility of the equation of state has broken down.

---

\* gjackland@ed.ac.uk

- [1] J. P. Perdew and A. Zunger, Phys. Rev. B **23**, 5048 (1981), URL <https://link.aps.org/doi/10.1103/PhysRevB.23.5048>.
- [2] J. P. Perdew, K. Burke, and M. Ernzerhof, Physical Review Letters **77**, 3865 (1996), URL <https://link.aps.org/doi/10.1103/PhysRevLett.77.3865>.
- [3] J. Sun, R. C. Remsing, Y. Zhang, Z. Sun, A. Ruzsinszky, H. Peng, Z. Yang, A. Paul, U. Waghmare, X. Wu, et al., Nature Chemistry **8**, 831 (2016), ISSN 1755-4349, URL <https://doi.org/10.1038/nchem.2535>.
- [4] P. Blaha, K. Schwarz, F. Tran, R. Laskowski, G. K. H. Madsen, and L. D. Marks, The Journal of Chemical Physics **152**, 074101 (2020), <https://doi.org/10.1063/1.5143061>, URL <https://doi.org/10.1063/1.5143061>.
- [5] G. N. Kamm and J. R. Anderson, Phys. Rev. B **2**, 2944 (1970), URL <https://link.aps.org/doi/10.1103/PhysRevB.2.2944>.
- [6] L. Dubrovinsky, N. Dubrovinskaia, E. Bykova, M. Bykov, V. Prakapenka, C. Prescher, K. Glazyrin, H.-P. Liermann, M. Hanfland, M. Ekholm, et al., Nature **525**, 226 (2015).
- [7] G. Kresse and J. Hafner, Phys. Rev. B **47**, 558 (1993), URL <https://link.aps.org/doi/10.1103/PhysRevB.47.558>.
- [8] G. Kresse and J. Furthmüller, Computational Materials Science **6**, 15 (1996), ISSN 0927-0256, URL <https://www.sciencedirect.com/science/article/pii/S0927025696000080>.

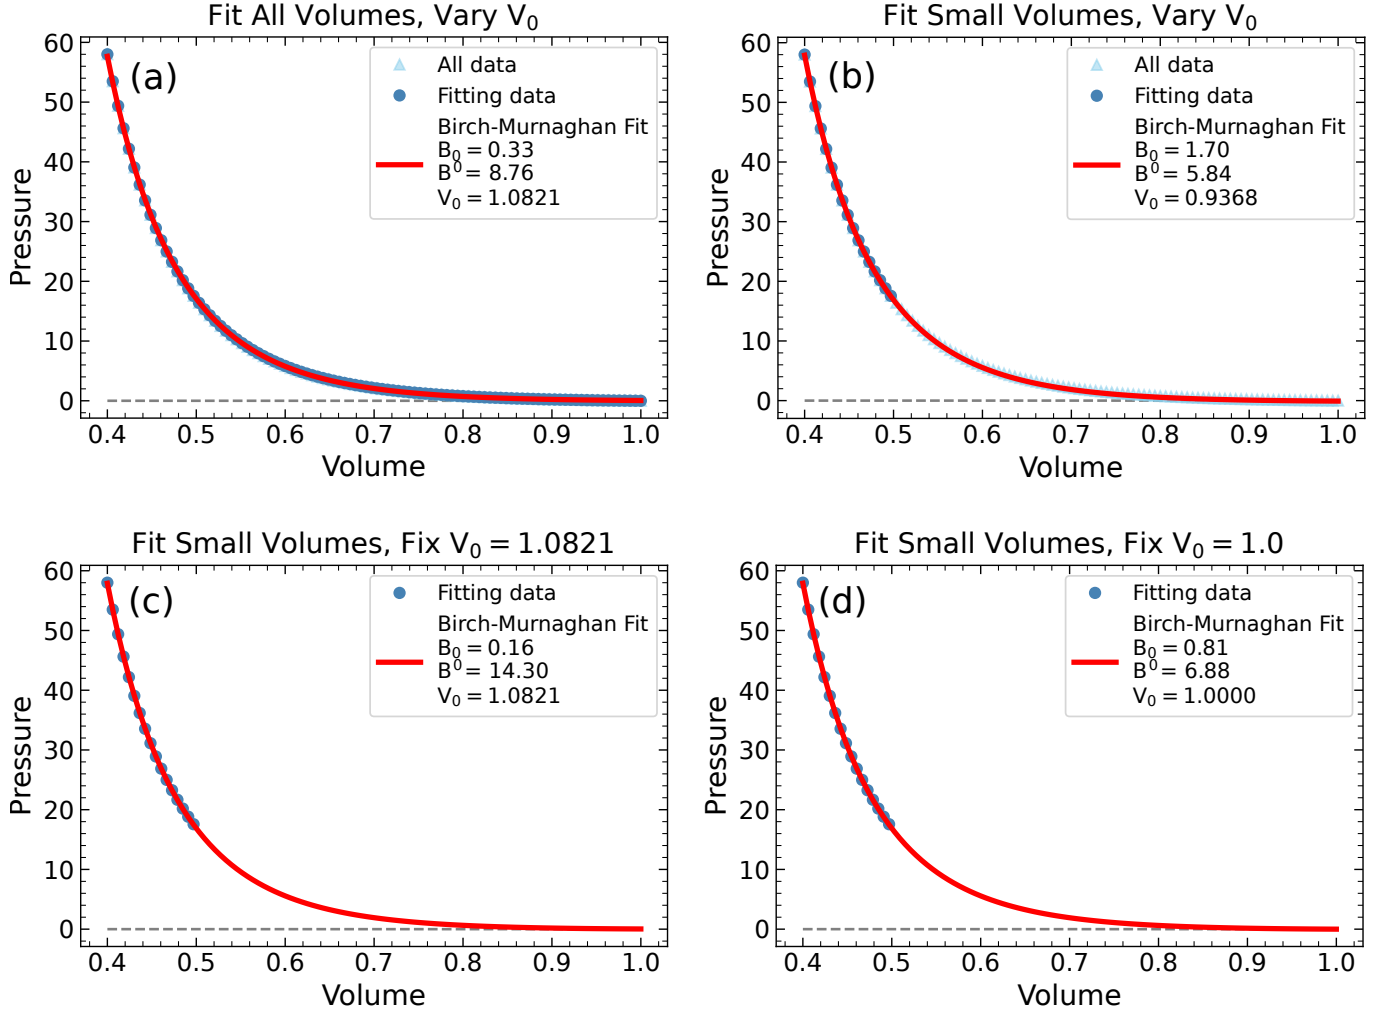

FIG. 16: Third-order Birch–Murnaghan equations of state fitted to pressure–volume data generated using a Lennard–Jones style equation of state (Eq. 2). (a) Fitted to all the generated data, (b) Fitted to just the data at volumes below 0.5, allowing  $V_0$  to vary, (c) Fitted only to low-volume data, but fixing  $V_0$  to the original fitted value of 1.0821, (d) Fitted only to low-volumes, and fixing  $V_0$  to the equilibrium value of 1.0.
